# Supplementary material for: STITCH: Augmented Dexterity for Suture Throws Including Thread Coordination and Handoffs
Source: arXiv:2404.05151 source file (2024-04-08)
Supplement: Supplementary file 1 [file section-7-appendix.tex]

\section{Appendix}

Appendix section can be added for the arxiv version of the paper.
